# Supplementary material for: A Dual Curriculum Learning Framework for Multi-UAV Pursuit-Evasion in Diverse Environments
Source: arXiv:2312.12255 source file (2024-04-30)
Supplement: Supplementary file 1 [file 70appendix.tex]

\todo{baselines details}
